# Supplementary material for: Influence of planets on debris discs in star clusters -- II. The impact of stellar density
Source: arXiv:2409.00996 source file (2024-09-02)
Supplement: Supplementary file 1 [file appendix.tex]

\appendix
\section{Appendix}
